# Supplementary material for: The Expressive Power of Transformers with Chain of Thought
Source: arXiv:2310.07923 source file (2024-04-11)
Supplement: Supplementary file 1 [file appendix-new.tex]

\section{Preliminaries} \label{sec:prelim}

We study the power of decoder-only transformers that can generate intermediate tokens between reading the input and generating an answer. On input $x \in \Sigma^n$, the transformer consumes tokens $x_1, \ldots, x_n$ for the first $n$ steps, and then, for $t(n)$ \emph{intermediate steps}, consumes the token generated by the previous step. At each step, the transformer can attend over all previous hidden states.
This standard method of generating text from a decoder-only model can be described formally as follows.
Let $\Sigma$ be a finite alphabet and $f : \Sigma^* \to \Sigma$ be a function mapping a prefix to a next token (parameterized by a transformer).
Let $\cdot$ be concatenation.
We define the $k$-step extension of $f$ as
\begin{align*}
    f^0(x) = x , \quad \quad \quad
    f^{k+1}(x) = f^k(x) \cdot f(f^k(x)) .
\end{align*}
We say we have run $f$ on $x$ with $t(n)$ (additional) decoding steps if we compute the function $f^{t(\abs{x})}(x)$. We consider $f$ with $t(n)$ steps to recognize the language of strings such that $f^{t(\abs{x})}(x) = 1$, where $1 \in \Sigma$ is a special ``accept'' symbol. We denote by $\CoT(t(n))$ the set of languages that are recognized by $t(n)$ decoding steps for some transformer $f$.
% We thus now turn to defining transformers.

\subsection{Transformers}

A transformer is a neural network parameterizing a function $\Sigma^* \to \Sigma$.
% We largely follow the definition of \citet{merrill2023logic,merrill2023parallelism}.
Let $\mathbb D_p$ be the datatype of $p$-precision floats and define $p$-truncated addition ($+, \sum$), multiplication ($\cdot$), and division ($/$) over $\mathbb D_p$ as in \citet{merrill2023parallelism}. We now define the high-level structure of the transformer in terms of its core components, with the details of those components in \Cref{sec:modules}.

\begin{definition}[\citealt{merrill2023logic}]
A $p$-precision decoder-only transformer with $h$ heads, $d$ layers, model dimension $m$ (divisible by $h$), and feedforward width $w$ is specified by:
\begin{compactenum}
    \item An embedding function $\phi : \Sigma \times \mathbb N \to \mathbb D_p^m$ whose form is defined in \Cref{sec:embedding};
    \item For each $1 \leq \ell \leq d$ and $1 \leq k \leq h$, a head similarity function $s^\ell_k : \mathbb D_p^m \times \mathbb D_p^m \to \mathbb D_p$ whose form is defined in \Cref{sec:self-attention};
    \item For each $1 \leq \ell \leq d$ and $1 \leq k \leq h$, a head value function $v^{\ell}_k : \mathbb D_p^m \to \mathbb D_p^{m/h}$ whose form is defined in \Cref{sec:self-attention};
    \item For each $1 \leq \ell \leq d$, an activation function $f^\ell : (\mathbb D_p^{m/h})^h \times \mathbb D_p^m \to \mathbb D_p^m$ whose form is defined in \Cref{sec:feedforward} and implicitly uses the feedforward dimension $w$;
    \item An output function $\gamma : \mathbb D_p^m \to \Sigma$ parameterized as a linear transformation.
\end{compactenum}
\end{definition}

\begin{definition} \label{def:transformer-computation}
We define one decoding step $\Sigma^n \to \Sigma$ with a decoder-only transformer as follows:
\begin{compactenum}
    \item \underline{Embeddings:} For $1 \leq i \leq n$, $\mathbf h^0_i = \phi(x_i, i)$.
    \item \underline{Multihead Self Attention:} For each layer $1 \leq \ell \leq d$, we compute $h$ attention heads:
    \begin{equation*}
        \mathbf a^{\ell}_{i,k} = \sum_{j=1}^i \frac{s^{\ell}_k(\mathbf h^{\ell-1}_i, \mathbf h^{\ell-1}_j)}{Z^\ell_{i,k}} \cdot v^{\ell}_k(\mathbf h^{\ell-1}_j) ,
        \quad \textrm{where} \;
        Z^\ell_{i,k} = \sum_{j=1}^i s^{\ell}_k(\mathbf h^{\ell-1}_i, \mathbf h^{\ell-1}_j) .
    \end{equation*}

    \item \underline{Activation Block:} For $1 \leq \ell \leq d$, activation block $\ell$ maps the head outputs to $\mathbf h^\ell$:
    \begin{equation*}
        \mathbf h^{\ell}_i = f^{\ell}(\mathbf a^{\ell}_{i,1}, \ldots, \mathbf a^{\ell}_{i,h}, \mathbf h^{\ell-1}_i) .
    \end{equation*}
    \item \underline{Classifier Head:} The transformer output is $\gamma(\mathbf h^d_n)$.
\end{compactenum}
\end{definition}

% We have now defined how a transformer parameterizes a function $\Sigma^* \to \Sigma$, and can thus be used as discussed above. A couple points remain to be clarified.

\paragraph{Transformer Precision.} We consider log-precision transformers \citep{merrill2023parallelism}, i.e., we allow the transformer at most $c \log m$ on $m$th decoding steps. As a transformer with intermediate generation runs for $n$ input steps and $t(n)$ intermediate decoding steps, this means we have precision at most $c \log(n + t(n))$.
Log precision is natural because it gives the the transformer just enough precision to represent indexes and sums across different positions, and it has then been analyzed in prior work \citep{perez2021attention,merrill2023parallelism,merrill2023logic}.

\paragraph{Saturation.} A saturated transformer \citep{merrill2021effects} is an idealized transformer with simple attention: all attention scores are either $0$ or $1/v$ for some $v$. Crucially, saturated attention can express full uniform attention ($1/n$ over $n$ positions) or hard attention (full weight on one position).
Our upper bounds do not require saturated attention, but, following common practice \citep{perez2021attention,merrill2023parallelism} we construct all our lower bounds using saturated attention. This shows that the constructions can be implemented without complicated attention patterns.

\subsection{Automata}

A deterministic finite-state automaton is a tuple $\langle \Sigma, Q, q_0, \delta, F \rangle$ where:

\begin{compactenum}
    \item $\Sigma$ is a finite input vocabulary
    \item $Q$ is a finite set of states containing initial state $q_0$
    \item $\delta$ is a transition function $Q \times \Sigma \to Q$
    \item $F \subseteq Q$ is a set of final states
\end{compactenum}

We define computation with an automaton on input string $\sigma \in \Sigma^*$ as follows.
An automaton configuration is simply a current finite state $q \in Q$.
We start with the initial state $q_0$.
We process a string $\sigma \in \Sigma^n$ one token at a time, computing the next state $q_i = \delta(q_{i-1}, \sigma_i)$ recurrently for $1 \leq i \leq n$.
% \begin{equation*}
%     q_i = \delta(q_{i-1}, \sigma_i) .
% \end{equation*}
We say that an automaton \emph{accepts} a string if $q_n \in F$ and that it \emph{rejects} it otherwise. The formal language that the automaton recognizes is the set of strings that it accepts.

\subsection{Turing Machines}

Adapting the notation of \citet{hopcroft2001introduction}, a multitape Turing machine is a tuple $\langle \Sigma, \Gamma,k, b, Q, q_0, \delta, F \rangle$ where:

\begin{compactenum}
    \item $\Sigma$ is a finite input vocabulary
    \item $\Gamma$ is a finite tape vocabulary with $\Sigma \subseteq \Gamma$
    \item $k$ is the number of work tapes
    \item $b$ is a blank symbol such that $b \in \Gamma$ and $b \not\in \Sigma$
    \item $Q$ is a finite set of states containing initial state $q_0$
    \item $\delta$ is a transition function $(Q \setminus F) \times \Gamma^{k+2} \to Q \times \Gamma^{k+1} \times \{\pm 1\}$
    \item $F \subseteq Q$ is a set of final states
\end{compactenum}

We define computation with a Turing machine on input string $\sigma \in \Sigma^*$ as follows.
A \emph{configuration} of a Turing machine is a finite state $q$ along with the contents of an input tape $c^0$, $k$ work tapes $c^1, \ldots, c^k$, and an output tape $c^{k+1}$. Finally, for each tape $\tau$, a configuration specifies a head position $h^\tau$.
We start with the initial state $q_0$ and the input tape $c^0_0$ containing $\sigma$ starting at position $0$ with infinite $b$'s on each side, and $h^0_0 = 0$.
All other tapes start containing all $b$'s and with their head at $0$. 
At each time step $i$, if $q_i \not\in F$, we recurrently update the configuration by first computing:
\begin{equation*}
    \langle q_{i+1}, \gamma^1_i, \ldots, \gamma^{k+1}_i, d^1_i, \ldots, d^{k+1}_i \rangle = \delta(q_i, c^0_i[h^0_i], \ldots, c^{k+1}_i[h^{k+1}_i]) .
\end{equation*}
We then update tape $\tau$ by setting $c^\tau_{i+1}[h^j_i] = \gamma^j_i$ and keeping all other tape cells the same. We update the head position on tape $\tau$ according to $h^\tau_{i+1} = h^\tau_i + d^\tau_i$.
On the other hand, if $q_i \in F$, we say the Turing machine halts and take as its output the string of tokens on the output tape from the current head position on the left up to (but not including) the first $b$ to its right. This shows how Turing machines parameterize functions $\Sigma^* \to \Sigma^*$.
A Turing machine can also be viewed as a language recognizer if we set $\Sigma = \{0, 1\}$ and check whether the first token of the output string is $0$ or $1$, constituting a language membership decision.

%%%%%%%%%%%%%%%%%%%%%
\section{Lower Bounds for Transformer Decoders}
\label{sec:lower-bounds}

Prior work \citep{merrill2023logic} has established strong upper bounds on the reasoning problems transformers can recognize. Specifically, accepting standard conjectures in complexity, transformers without intermediate decoding cannot recognize all regular languages.

In this section, we show that some of these shortcomings can be addressed with a suitable number of intermediate decoding steps. Specifically, a linear number of steps is sufficient to simulate an automaton. We also show how this construction can be extended so that a transformer with $t(n)$ intermediate decoding steps can simulate a Turing machine for $t(n)$ steps.

\subsection{Introducing Layer-Norm Hash} \label{sec:lnorm-hash}

We first introduce a useful building block for our results that we call the \emph{layer-norm hash}. The layer-norm hash is a mechanism that enables retrieval across different columns in the transformer based on query-key matching of numerical values.
Exact-match retrieval is trivial when the query $q_i$ and keys $k_1, \ldots k_i$ are items in a finite set: just one-hot encode $q_i$ and $k_j$ and the inner product will be maximized when $q_i$ and $k_j$ match.
This does not work, though, when the keys and values are counts produced by uniform attention, which many transformer algorithms use \citep{weiss2021thinking}.
In this case, the key is a fraction $q_i/i$ and the queries are fractions $k_j/j$ with \emph{diferent} denominators.

The layer-norm hash helps by representing $q_i/i$ and $k_j/j$ such that hard attention retrieves the value $j$ where $q_i = k_j$. The idea is to use layer-norm to project $q_i$ and $k_j$ to vectors $\phi_{q_i}$ and $\phi_{k_i}$ on the unit sphere satisfying this property.
% where $\mathbf \phi_{q_i}^\top \cdot \phi_{k_j} = 0$ if and only if $q = k$.
Let $\lnorm(\mathbf x)  = \frac{\mathbf x'}{\norm{\mathbf x'}}$, where $\mathbf x' = \mathbf x - \bar x$.

% The layer-norm hash is a useful function computable by a transformer that enables comparing absolute counts between different columns in the transformer. Concretely, imagine $q/n$ is a fraction computed by taking uniform attention over $n$ previous positions. For any $q \in \mathbb R$, $n \in \mathbb N$, the layer-norm hash is a vector representation of this scalar:

\begin{definition}[Layer-norm hash]
    Given a scalar $x \in \mathbb R$, its layer-norm hash at position $i \in \mathbb N$ is
    \begin{equation*}
        \hash(x/i, 1/i) = \lnorm \left( \frac{x}{i}, \frac{1}{i}, -\frac{x}{i}, -\frac{1}{i} \right) .
    \end{equation*}
\end{definition}

This is a unit vector in $\mathbb R^4$. A key feature of this representation is that it is invariant w.r.t.\ $i$ in the sense that $\hash(x/i, 1/i)$ is only a function of $x$, independent of $i$.
Let $\hash_x \triangleq \hash(x, 1)$:
\begin{restatable}[Proof in \Cref{sec:lnorm-proof}]{lemma}{lnormcanonical} \label{lem:lnorm-canonical}
    For any $x \in \mathbb{R}$ and $i \in \mathbb{N}$, $\hash(x/i, 1/i) = \hash_x$.
\end{restatable}
Further, the inner products of these representations of two scalars $q, k$ checks equality of $q$ and $k$:
\begin{restatable}[Proof in \Cref{sec:lnorm-proof}]{lemma}{lnormunique} \label{lem:lnorm-unique}
    For any $q, k \in \mathbb R$, $\phi_q \cdot \phi_k = 1$ if and only if $q = k$.
\end{restatable}

% \begin{restatable}{lemma}{lnormhash} \label{lem:lnorm-hash}
%     For $q, k \in \mathbb{R}, i, j \in \mathbb N$, $\hash(q/i, 1/i) \cdot \hash(k/j, 1/j)$ is maximized exactly when $q = k$.
% \end{restatable}

We can look up key $q_i/i$ in a sequence of keys $k_1/1, \ldots, k_i/i$ by attending with query $\hash(q_i/i, 1/i)$ at position $i$ and key $\hash(k_j/j, 1/j)$ at each $j$.
By \Cref{lem:lnorm-canonical,lem:lnorm-unique} this retrieves the value at $j$ such that $q_i = k_j$.
The layer-norm hash can also be used to directly compare two values $q_i, k_j$ without removing the denominator by computing $\hash(q_i, 1)$ and $\hash(k_j, 1)$.

The first use of the layer-norm hash requires having $1/i$ at position $i$. \Cref{lem:start-separable} shows that a transformer decoder can compute $1/i$ at each position $i$ assuming start-separable positional encodings:

\begin{definition}
    A positional encoding $\pi$ is \textbf{start-separable} if there exists a transformer decoder that maps the position embedding sequence to $\langle 1, 0, \ldots, 0 \rangle$ (i.e., tags whether each token is the first).
\end{definition}

The initial token is always separable if there is a special \texttt{bos} token. Similarly, if the position embedding of $1$ is unique, then the initial token is separable. Since one of these conditions will likely be met in practice, we believe any practical transformer variant should be start-separable.\footnote{Technically it will repeat for sinusoidal positional encodings, but not on inputs with in-domain length.} By \Cref{lem:start-separable} can effectively ``reduce'' these other positional encodings to $1/i$ encodings: any construction with $1/i$ positional encodings can be adapted to work for any start-separable encoding.
% \ashish{currently the copy of this lemma in the appendix is called Lemma 5.  Can either drop that (just have the proof there) or renumber that} \will{lemma 2 for me?}

\begin{restatable}[Proof in \Cref{sec:start-separable}]{lemma}{startseparable} \label{lem:start-separable}
    For any language $L$,
    if some decoder-only saturated transformer with $1/i$ positional encodings recognizes $L$, then,
    for any start-separable positional encoding $\pi$, some decoder-only saturated transformer with $\pi$ positional encodings recognizes $L$.
\end{restatable}

\subsection{Simulating Automata}

We can use the layer-norm hash to simulate models of computation like automata or Turing machines with intermediate-generation transformers. To warm up, we first show how to use the layer-norm hash to simulate an automaton (i.e., recognize a regular language) and then extend it in \Cref{sec:turing-machine} to show how a transformer can simulate a Turing machine for a bounded number of steps.

\begin{theorem} \label{thm:automata}
    Let $L$ be a regular language.
    For any start-separable positional encoding,
    there is a decoder-only saturated transformer
    that recognizes whether $x \in L$ with $\abs{x} + 1$ decoding steps.
\end{theorem}

\begin{proof}
Without loss of generality, we construct a transformer with $1/i$ positional encodings (cf. \Cref{lem:start-separable}).
The idea is to simulate one step of the automaton with one transformer decoding step (after first reading $n$ input tokens). At decoding step $i$, we will output a token $q_i$ encoding the state transitioned to. After printing the final state $q_n$, we use one additional step to output $1$ iff $q_n \in F$.

The base case of $i=0$ corresponds to the final input token, at which we output the initial state $q_0$.

In the inductive case, we know that the sequence of intermediate tokens is $q_0, \ldots, q_i$. Our goal is to compute and output $q_{i+1} = \delta(q_i, \sigma_i)$, which first involves computing $\delta$'s two arguments. We already have $q_i$ as the input to the current column of the transformer.
We use hard attention to retrieve the current input symbol $\sigma_{i+1}$. We already have $1/j$ stored at each input position $j$. Decoding step $i+1$ corresponds to the $(n + i + 1)$st input to the transformer. We attend uniformly over the left context with a value of $1$ at decoding steps and $0$ at input steps, yielding $1/(i + 1)$. We attend with query $\hash(1/(i+1), 1)$, keys $\hash(1/j, 1)$, and values $\sigma_j$. By \Cref{lem:lnorm-unique}, attention is maximized at $j = i + 1$, so this head retrieves $\sigma_{i+1}$.
At this point, we have the current finite state $q_i$ and current input token $\sigma_{i+1}$. We conclude by using a feedforward network to output $q_{i+1} = \delta(q_i, \sigma_{i+1})$.
\end{proof}

\Cref{thm:automata} shows that a linear number of decoding steps gives additional reasoning power to log-precision transformers (assuming $\TC^0 \neq \NC^1$).
This follows because log-precision transformers with no decoding steps are contained in uniform $\TC^0$ \citep{merrill2023parallelism}, which means they cannot recognize all regular languages. In contrast, \Cref{thm:automata} says a linear number of steps is sufficient for recognizing all regular languages, establishing a conditional separation.

\Cref{thm:automata} shows an example of simple and familiar additional computational power granted by additional decoding steps.
The core challenge in simulatingan automaton is simulating recurrence, which cannot be done without decoding steps \citep{merrill2023parallelism}. Intuitively, a linear number decoding steps is sufficient for simulating recurrence, which is where the additional power comes from.
However, this additional power does not stop with finite-state machines: the layer-norm hash can be used to simulate more complex models of computations like Turing machines, which we will turn to in the next section.

\subsection{Simulating Turing Machines} \label{sec:turing-machine}

We now show that the layer-norm hash can be applied to construct a transformer decoder that uses $t(n)$ intermediate steps to simulate a Turing machine for $t(n)$ steps. Our decoder-only construction resembles the encoder-decoder construction of \citet{perez2021attention} for simulating Turing machines. However, it avoids a simplifying assumption from \citet{perez2021attention}: they needed the transformer to have access to $1/i, 1/i^2,$ and $i$ in its positional embeddings. This assumption is problematic because transformers cannot represent unbounded scalars like $i$ due to layer-norm and it is unclear how a transformer could compute a square like $1/i^2$. In contrast, our construction works for any start-separable positional encoding, including just $1/i$.

\begin{theorem} \label{thm:lower-bound}
    Let $M$ be a Turing machine that, on input length $n$, runs for at most $t(n)$ steps.
    % Let $\pi$ be a positional encoding scheme that allows separating the first token.
    % Then 
    For any start-separable positional encoding,
    there exists a decoder-only saturated transformer that, on input $x$, computes $M(x)$ with $t(n) + \abs{M(x)}$ decoding steps.
\end{theorem}

\begin{proof}
    Without loss of generality, we show a construction for transformers with $1/i$ positional encodings (cf. \Cref{lem:start-separable}).
    We will construct a transformer decoder that simulates a Turing machine in real time, i.e., a single transformer decoding step will simulate one Turing machine step. This means the simulation will take $t(n)$ steps, followed by an additional $\ell(n)$ steps to reconstruct the output. The main difficulty will be constructing a distributed representation of a Turing machine tape in a sequence of transformer state vectors and showing how the transformer can both maintain this representation and correctly reconstruct the current status of the tape at the head position. The key idea to the construction will be to store ``diffs'' to the tape at each timestep and use the layer-norm hash to dynamically reconstruct the contents at the head position at every new timestep.

    We introduce a new finite vocabulary $\Delta$ and identify each element of $Q \times \Gamma \times \{\pm 1 \}$ with some $\delta \in \Delta$. A deterministic Turing machine run of length $m$ induces a \emph{diff sequence} $\delta_0, \ldots, \delta_m \in \Delta$ capturing the state entered, token written, and direction moved after each token.
    % The diff sequence encodes all the information necessary to accept or reject a string with a Turing machine: simply project $\delta_i$ onto its first component $q_i$ and check whether $q_i \in F$.
    We show by induction over $i$ that we can output $\delta_i$ at decoding step $i$:

    % \begin{compactenum}
        % \item 
        \underline{Base Case:} In the first layer of the transformer, we use a different head to reconstruct the current position on each tape. At each position $i$, the head attends uniformly over the full left context where the value at a decoding step $j$ is the $(\tau + 1)$st component of $\delta_j$, corresponding to $d^\tau_j$, the move direction on tape $\tau$ at time $j$.\footnote{Let the attention value be $0$ at an input step. This construction can be easily extended to allow no-op moves.} The value of this head is thus $h^\tau_i/(n+i)$, where $h^\tau_i$ is the position on tape $\tau$ after $i$ steps.

        % \item 
        \underline{Inductive Case:} We can now apply $k$ different layer-norm hashes to get $\phi^\tau_i = \hash(h^\tau_i/(n+1), 1/(n+i))$ in parallel at each $i$. By \Cref{lem:lnorm-unique}, the inner product $\phi^\tau_i \cdot \phi^\tau_j$ is maximized when $h^\tau_i$ and $h^\tau_j$ are equal. For each $\tau$ we construct a head that hard-attends with query $\langle \phi^\tau_i, 0 \rangle$ over keys $\langle \phi^\tau_j, -1/j \rangle$ and values $\delta_{h^\tau_j}$, for $j \leq i$. This returns the last update $d^\tau_i$ written to the head position at step $i$.

        We now have all necessary inputs to compute the next Turing machine transition.
        For each $\tau$, the second component of $d^\tau_i$ is $\gamma^\tau_i$: the current contents of cell $h^\tau_i$ of tape $\tau$. As input to column $i$ of the transformer, we have $\delta_{i - 1}$, which contains $q_{i-1}$. We now compute
        % \begin{equation*}
            $\delta_i = \delta(q_{i-1}, \gamma^0_i, \ldots \gamma^{k + 1}_i)$
        % \end{equation*}
        using a feedforward network, which is possible because this computation is simply a finite table lookup. We write out $\delta_i$ as the output of the column, completing the inductive step.
    % \end{compactenum}

    Finally, we use at most $\ell(n)$ additional steps to reconstruct the Turing machine output. Analogously to above, we retrieve $d^{k+1}_i$, the last update written to the current head position on the output tape, and output $\gamma^{k+1}_i$. We then write a diff $\delta_i$ that moves the head to the right. We iterate in this state until $b$ (blank) is read, at which point we halt.
    We conclude that we are able to simulate $M$ in real-time, i.e., the transformer runs one decoding step per step of $M$ followed immediately by $M$'s output.
\end{proof}

% \Cref{thm:lower-bound} gives a lower bound on the expressive power of transformer decoders with $t(n)$ steps:
\begin{corollary} \label{cor:lower-bound}
    $\TIME(t(n)) \subseteq \CoT(t(n))$.
\end{corollary}
% We thus see that we can more efficiently simulate a Turing machine compared to the slow simulation derived via counter automata in \Cref{thm:counter-automata}.
This lets us reason about the power of transformer decoders in terms of Turing machines.
We see simulating an automaton (cf.~\Cref{thm:automata}) is not the only new capability unlocked with $\O(n)$ steps: rather, we can solve \emph{any} problem a Turing machine can solve in $\O(n)$ time, such as simulating real-time counter machines.\footnote{A memory-augmented variant of finite automata similar to LSTMs \citep{weiss2018practical}.}
With $\O(n^2)$ steps, we can run an $\O(n^2)$-time Turing machine to solve directed graph connectivity using standard graph traversal methods like depth-first search. These methods run in $\O(n)$ time on a random access Turing machine~\citep{wigderson1992complexity}, which can be simulated in $\O(n^2)$ time without random access.
It is possible that transformer decoders can solve directed graph connectivity with fewer than $\O(n^2)$ steps, as results from \citet{zhang2023language} hint at.
% or solve directed graph connectivity \citep{wigderson1992complexity}.

% With polynomial steps, \Cref{thm:lower-bound} implies transformer decoders can recognize all of $\P$, similar to past results for encoder-decoder models \citep{perez2021attention}.  While this means a polynomial number of decoding steps makes transformers quite expressive, it is likely infeasible to run large transformers for this many steps in practice.
% , and there are no guarantees that transformer decoders will \emph{learn} to simulate Turing machines, especially in a way that will generalize to long inputs.

%%%%%%%%%%%%%%%
\section{Upper Bounds for Transformer Decoders}
\label{sec:upper-bounds}

Having shown lower bounds on transformer with $t(n)$ steps,
we present two different upper bounds: one that relates transformer decoders to time complexity classes, and one that relates them to space complexity classes. The relative strength of the two different bounds will vary depending on $t(n)$.

% we will now extend the results of \citet{merrill2023parallelism} to upper bound on the languages recognized by transformers with $t(n)$ decoder steps.

\subsection{Time Upper Bound}

A simple upper bound on transformers with chain of thought can be obtained based on the fact that transformers can be simulated using a quadratic number of arithmetic operations.

\begin{theorem} \label{thm:naive-upper-bound}
    $\CoT(t(n)) \subseteq \tildeTIME(n^2 + t(n)^2)$.
\end{theorem}
\begin{proof}
We sketch a multitape Turing machine that will simulate the transformer. Each forward pass $i$ appends key $i$ onto a work tape and value $i$ onto another work tape. To simulate the forward pass at time $i$, it suffices to show how to simulate computing self-attention at time $i$.

To compute self attention, the Turing machine first computes the query at time $i$. It then iterates over pairs on the key and value work tapes. For each pair $j$, we compute the attention score between query $i$ and key $j$ and then multiply it by value $j$ using additional work tapes. We then add this value to a running sum tape.
We treat the final sum at the output of the attention mechanism.

For runtime, observe that we compute $n + t(n)$ forward passes, and each forward pass involves looping over $n + t(n)$ key-value pairs. This means we run at most $\O(n^2 + t(n)^2)$ inner loop calls.
It remains to be shown that one inner loop runs in polylogarithmic time.
An inner loop just involves adding and multiplying $\O(\log n)$-bit numbers.
$p$-bit numbers can be added in time $\O(p) = \O(\log n)$.
Similarly, $p$-bit numbers can be multiplied in time $\O(p \log p) \leq \O(p^2)$, which comes out to $\log^2 (n + t(n))$ with log precision.
Thus, one inner loop can be run in polylogarithmic time.
We conclude that a transformer decoder with $t(n)$ intermediate steps can be simulated by a multitape Turing machine in time $\tildeO(n^2 + t(n)^2)$.
\end{proof}

\subsection{Space Upper Bound}

Our second upper bound relies on the $\TC^0$ upper bound for transformers without intermediate steps.

\begin{theorem} \label{thm:space-ub}
    $\CoT(t(n)) \subseteq \SPACE(t(n) + \log n)$.
\end{theorem}

\begin{proof}
    % Let $h$ be a function such that we can simulate a transformer on inputs of size $n$ using at most $h(n)$ space \ashish{since we aren't going for a lower bound based on $h$, might be simpler to directly say: By prior paper ..., we know transformers can be simulated in $\L$ and thus in space $h(n) = c \log n$ for some $c$.}.
    Since log-precision transformers can be simulated in uniform $\TC^0$ \citep{merrill2023parallelism}, they can be simulated in $\L$, i.e., with at most $c \log n$ space overhead on inputs of size $n$.
    % We thus know there is some $c$ such that $h(n) = c \log n$.

    To compute $t(n)$ intermediate decoding steps of a transformer, we store a buffer of at most $t(n)$ generated tokens, which has size $\O(t(n))$. To compute the next token, we call the transformer with an input of size $\O(n + t(n))$ using at most $c \log(n + t(n))$ space overhead.
    % , as noted above.
    We then clear the memory used and append the finite token generated to the input buffer.
    It follows from this algorithm that
    \begin{equation*}
        \CoT(t(n)) \subseteq \SPACE(t(n) + c \log(n + t(n))) .
    \end{equation*}
    Since $\log$ is subadditive, we can simplify:
    \begin{align*}
        \CoT(t(n))
        &\subseteq \SPACE(t(n) + c \log n + c \log t(n)) \\
        &= \SPACE(t(n) + \log n) . \qedhere
    \end{align*}
\end{proof}

With at least $\Omega(\log n)$ steps, this upper bound can be simplified to $\SPACE(t(n))$.
The $t(n) = \Theta(n)$ case establishes the context-sensitive languages as an upper bound for transformers with linear steps.
Given our $\TIME(t(n))$ lower bound~(\Cref{thm:lower-bound}), the tightest possible space upper bound without making fundamental complexity advances would be $\SPACE(t(n) / \log t(n))$ \citep{Hopcroft1977OnTV}. Conversely, our lower bound can only be tightened to $\TIME(t(n) \log t(n))$.

On the other hand, if we have only $\O(\log n)$ decoding steps, we see that intermediate decoding does not increase expressive power much beyond $\TC^0$, because the upper bound simplifies to $\SPACE(t(n)) = \L$.
Thus, under standard assumptions, transformers with at most a logarithmic number of decoding steps cannot solve directed graph connectivity, Horn formula satisfiability, or other $\NL$- or $\P$-complete problems. On the other hand, they may be able to solve $\L$-complete problems, unlike transformers without intermediate decoding.
